# Supplementary material for: Bound States in the Continuum in Multipolar Lattices
Source: arXiv:2202.10392 ancillary file (2022-02-22)
Supplement: Supplementary file 1 [file supplementary.pdf]

# Supplemental material: Bound States in the Continuum in Multipolar Lattices

Sergei Gladyshev, Artem Shalev, Kristina Frizyuk, Konstantin Ladutenko, and Andrey Bogdanov*
*School of Physics and Engineering, ITMO University, 191002, St. Petersburg, Russia*

Here we (i) provide the definitions of the vector spherical harmonics and spherical vectors that we used in the main text; (ii) compare the reflection and polarization maps for electric and magnetic octupolar lattices (Fig. S2) and recall the conditions of opening diffraction channel that is important for the formation of off-Γ BICs; (iii) derive the analytical expression for the radiative Q-factor of the leaky modes in multipolar lattice applicable in the whole Brillouin zone and compare it with numerical simulation (Fig. S3); (iv) derive equation (1) from the main text; (v) demonstrate the collective anapole state in multipolar lattice (Fig. S5), and, finally, (vi) present details of the modifications of the original code MULTEM which allows to simulate the reflection maps of multipolar lattices .

## S1.DEFINITION OF VECTOR SPHERICAL HARMONICS AND SPHERICAL VECTORS

Any electromagnetic field in three-dimensional problem can be expand into a series vector spherical harmonic (VSH)[1]

$$\mathbf{E}(\mathbf{r}) = \sum_s D_s \mathbf{W}_s(\mathbf{r}) \exp(i\mathbf{k}_b \cdot \mathbf{r}), \tag{1}$$

where $\mathbf{W}_s = \{\mathbf{N}_s, \mathbf{M}_s\}$ is the vector spherical harmonic. Index $s$ is a set of indices p,m,l. Index $l = 0, 1, 2, ...$ is the total angular momentum quantum number, and $m = 0, 1, ..., l$ is the absolute value of the projection of the angular momentum (magnetic quantum number). Index $p = \pm 1$ defines the parity of $\mathbf{W}_s$ with respect to reflection from the $xz$-plane ($\varphi \to -\varphi$). If $p = \pm 1$ then $\mathbf{W}_s \to \pm \mathbf{W}_s$ under reflection form the $xz$-plane. Let us note that this definition of parity differs from that given in Ref. [2].

$$\mathbf{M}_{-pml} = \nabla \times (\mathbf{r}\psi_{pml}), \tag{2}$$

$$\mathbf{N}_{pml} = \frac{\nabla \times \mathbf{M}_{-pml}}{k}, \tag{3}$$

$$\tag{4}$$

where

$$\psi_{1ml}(kr) = z_l(kr) P_l^m(\cos\theta)\cos m\phi, \tag{5}$$

$$\psi_{-1ml}(kr) = z_l(kr) P_l^m(\cos\theta)\sin m\phi. \tag{6}$$

Here $z_l(kr)$ can be replaced by the spherical Bessel, Neumann, or Hankel function and $P_l^m(\cos\theta)$ is the associated Legendre polynomial.

Spherical vectors $\mathbf{Y}_s = \{\mathbf{X}_s, \mathbf{Z}_s\}$ defined as

$$\mathbf{X}_{-pml}\left(\frac{\mathbf{k}}{k}\right) = \nabla \times \left[\mathbf{k} Y_{pml}\left(\frac{\mathbf{k}}{k}\right)\right], \tag{7}$$

$$\mathbf{Z}_{pml}\left(\frac{\mathbf{k}}{k}\right) = i\frac{\mathbf{k}}{k} \times \mathbf{X}_{-pml}\left(\frac{\mathbf{k}}{k}\right), \tag{8}$$

where

$$Y_{1ml}(\theta, \varphi) = \cos m\varphi P_l^m(\cos\theta), \tag{9}$$

$$Y_{-1ml}(\theta, \varphi) = \sin m\varphi P_l^m(\cos\theta). \tag{10}$$

Here $p = (-1)^{l+1}$ for $\mathbf{X}$, and $p = (-1)^l$ for $\mathbf{Z}$. Note that the transformation behavior is similar for $\mathbf{W}$ and $\mathbf{Y}, \mathbf{X}$ and $\mathbf{M}$, $\mathbf{Z}$ and $\mathbf{N}$, and $\psi$ and $Y$.

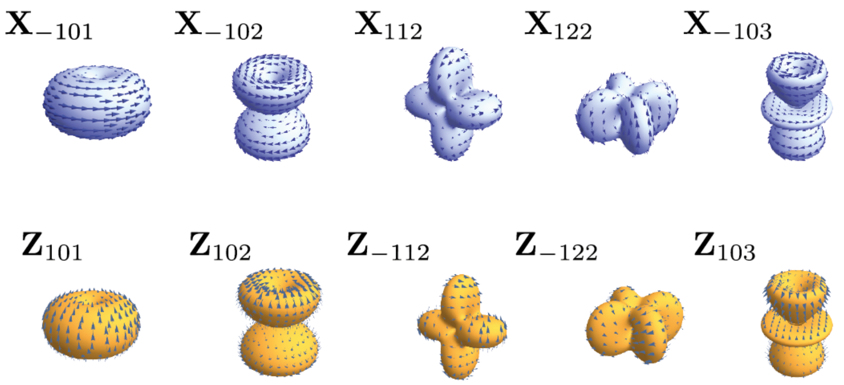


FIG. S1: Different spherical vectors $\mathbf{Y}_s = \{\mathbf{X}_s, \mathbf{Z}_s\}$ which describe the far-field of multipoles.

## S2. MULTIPOLAR LATTICES COMPOSED OF ELECTRIC AND MAGNETIC MULTIPOLES OF THE SAME ORDER

The electric and magnetic multipoles of the same order have the same intensity distribution in the far-field but different polarization structure (see Fig. S1). Figures S2 shows the reflection maps [panels (b) and (d)] and polarization maps [panels (c) and (e)] calculated for the electric octupolar ($\mathbf{Z}_{103}$) and magnetic octupolar ($\mathbf{X}_{-103}$) lattices shown schematically in Fig. S2(a). Parameters of the dielectric spheres emulating the multipoles are mentioned in the caption. The angular positions of the off-Γ BICs is the same as the far-field of the multipoles is described by the same functions.

One of the main conditions for the formation of off-Γ BIC is subwavelength regime. It is necessary that the condition on the relationship between mode frequency and position of BIC in k space must be satisfied

$$\begin{array}{l} k_z^2 = k_0^2 - (k_x - 2\pi m/a)^2 \\ k_0^2 - (k_x - 2\pi m/a)^2 = 0 \\ k_x/k_0 - 2\pi/ak_0 = 1 \end{array} \Rightarrow \frac{1}{1+\sin\theta} = \frac{\omega a}{2\pi c} = \tilde{\omega} \tag{11}$$

Therefore we need to choose the ratio $a/d$ and material for the sphere to satisfy the condition

$$\tilde{\omega} < \frac{1}{1+\sin\theta_0}, \tag{12}$$

where $\theta_0$ is the angle which characterizes the nodal line of $\mathbf{Y}_s$, $a$ and $d$ are the period and diameter, respectively.

## S3. ANALYTICS OF RADIATIVE Q-FACTOR IN MULTIPOLAR LATTICES

The definition of quality factor ($Q$) is the ratio of the energy stored in the system to the power loss. We consider the high-refractive index paricles in the systems and think that the internal energy stored in the particles is much greater than the external energy stored outside the particles.

$$\begin{aligned} Q &= \omega \frac{W_{\text{int}}^{\text{st}} + W_{\text{ext}}^{st}}{P_{\text{rad}}} = \omega \frac{W_{\text{int}}^{st}}{P_{\text{rad}}} \\ W_{\text{int}}^{\text{st}} &= \int_V \frac{1}{2} \left( \varepsilon \mathbf{E}\cdot\mathbf{E}^* + \mu \mathbf{H}\cdot\mathbf{H}^* \right) dV \end{aligned} \tag{13}$$

The radiated power loss of the system

$$P_{\text{rad}} = \frac{1}{2}\sqrt{\frac{\varepsilon_0}{\mu_0}} \frac{S_b^2 S_u}{4\pi^2 k_1^2 k_{1z}^2} \left| \tilde{D}_s \left[ \mathbf{Y}_s \left( \frac{\mathbf{k}_1}{k_1} \right) \right] \right|^2 \tag{14}$$

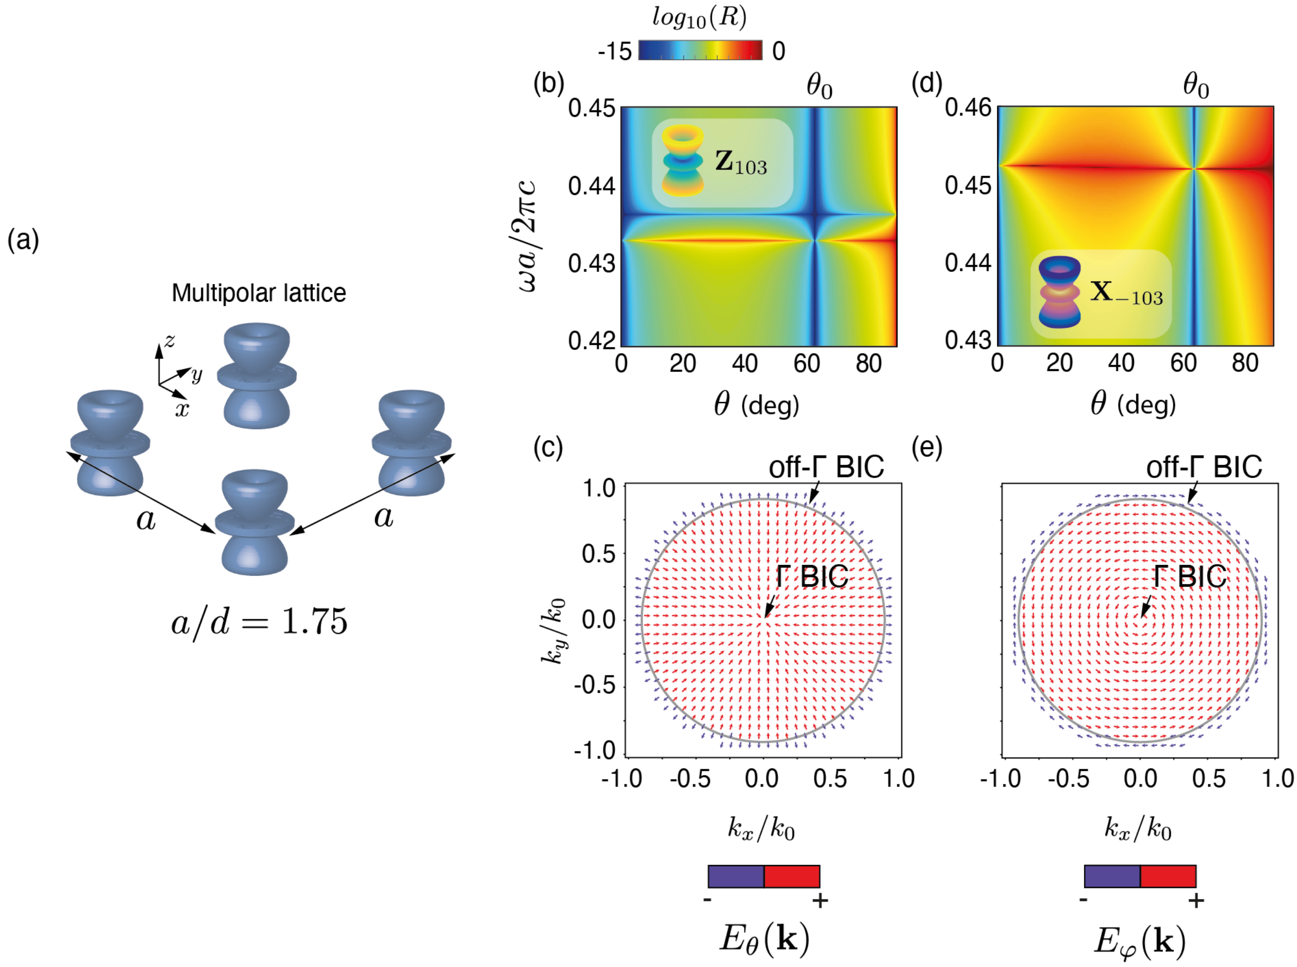


FIG. S2: (a) Multipolar lattice with the square unit cell and period $a$ containing a single multipole in the unit cell (electric $\mathbf{Z}_{tm\ell}$ or magnetic $\mathbf{X}_{tm\ell}$). (b) and (d) The reflection $R$ from the magnetic end electric octupolar lattice with a square plotted as a function of dimensionless frequency $\omega a/2\pi c$ and angle of incidence $\theta$ for the ration $a/d = 1.75$ in logarithmic scale. The magnetic octupole $\mathbf{X}_{-103}$ and electric octupole $\mathbf{Z}_{103}$ is described by the T-matrix of a high-refractive-index sphere neglecting all its scattering channels except the magnetic and electric octupolar, respectively. The permittivities of the sphere are $\varepsilon = 80$ and $\varepsilon = 50$ for electric and magnetic octupolar lattice, respectively. (c) and (e) Polarization map of the magnetic ($\mathbf{X}_{-103}$) and electric ($\mathbf{Z}_{103}$) multipolar band in the far-field showing the BICs forming a close continues line in the $k$-space. respectively.

where $S_u$ is unit cell area.

Field inside the nanoparticle

$$\mathbf{E}^{\text{in}}(\mathbf{r}) = \left[D_s \mathbf{W}_s^{(1)}(k_2, \mathbf{r}') \exp(i\mathbf{k}_b \cdot \mathbf{r}_j)\right] \tag{15}$$

where $\mathbf{r}' = \mathbf{r} - \mathbf{r}_j$ and $\mathbf{r}_j$ is the position of a single sphere.

The coefficients $D^h$ in (15) and $\tilde{D}^h$ in (14) are connected by the formula (where $h$ is index, which can be $\mathbf{N}$ or $\mathbf{M}$ belong to electric or magnetic multipole, respectively. )

$$\begin{aligned} \tilde{D}_s^M =& iD_s^M r_s^2 \varepsilon_1 \left[k_1^2 j_{l-1}(k_1 r_s) j_l(k_2 r_s) \right. \\ & \left. -k_1 k_2 j_{l-1}(k_2 r_s) j_l(k_1 r_s)\right] \end{aligned} \tag{16}$$

$$\begin{aligned}\tilde{D}_s^N =& iD_s^N r_s^2 \varepsilon_1 \left\{ \frac{l+1}{2l+1} \left[ k_1^2 j_{l-2}(k_1 r_s) j_{l-1}(k_2 r_s) \right.\right. \\ & \left. -k_1 k_2 j_{l-2}(k_2 r_s) j_{l-1}(k_1 r_s) \right] \\ & + \frac{l}{2l+1} \left[ k_1^2 j_l(k_1 r_s) j_{l+1}(k_2 r_s) \right. \\ & \left.\left. -k_1 k_2 j_l(k_2 r_s) j_{l+1}(k_1 r_s) \right] \right\}\end{aligned} \tag{17}$$

where $r_s$ is radius of the sphere.

The internal energy stored in the particles for magnetic ($\mathbf{M}$) multipole

$$\begin{aligned} W^{\text{st}}_{\text{int, M}} &= \varepsilon\varepsilon_0 \int_V \left| D_s \mathbf{M}_s^{(1)} \right|^2 dV = \\ \varepsilon\varepsilon_0 \left| D_s \right|^2 (1+\delta) & \frac{2\pi}{2l+1} \frac{(l+m)!}{(l-m)!} l(l+1) \cdot \\ \cdot \frac{r_s^3}{2} & \left( j_l(k_2 r_s)^2 - j_{l-1}(k_2 r_s) j_{l+1}(k_2 r_s) \right) \end{aligned} \tag{18}$$

The internal energy stored in the particles for electric ($\mathbf{N}$) multipole

$$\begin{aligned} W^{\text{st}}_{\text{int, N}} &= \varepsilon\varepsilon_0 \int_V \left| D_s \mathbf{N}_s^{(1)} \right|^2 dV = \\ \varepsilon\varepsilon_0 \left| D_s \right|^2 (1+\delta) & \frac{2\pi}{(2l+1)^2} \frac{(l+m)!}{(l-m)!} l(l+1) \\ \cdot \Bigg( (l+1) \frac{r_s^3}{2} & \left( j_{l-1}(k_2 r_s)^2 - j_{l-2}(k_2 r_s) j_l(k_2 r_s) \right) + \\ + l \frac{r_s^3}{2} & \left( j_{l+1}(k_2 r_s)^2 - j_l(k_2 r_s) j_{l+2}(k_2 r_s) \right) \Bigg) \end{aligned} \tag{19}$$

$$\begin{aligned} & \int_0^{2\pi} \int_0^{\pi} \mathbf{M}_{{}^1_{-1}ml} \cdot \mathbf{M}_{{}^1_{-1}ml} \sin\theta d\theta d\phi \\ &= (1+\delta) \frac{2\pi}{2n+1} \frac{(l+m)!}{(l-m)!} l(l+1) \left[ z_l(kR) \right]^2 \end{aligned} \tag{20}$$

$$\begin{aligned} & \int_0^{2\pi} \int_0^{\pi} \mathbf{N}_{{}^1_{-1}ml} \cdot \mathbf{N}_{{}^1_{-1}ml} \sin\theta d\theta d\phi \\ &= (1+\delta) \frac{2\pi}{(2n+1)^2} \frac{(l+m)!}{(l-m)!} l(l+1) \\ & \left\{ (l+1) \left[ z_{l-1}(kR) \right]^2 + l \left[ z_{l+1}(kR) \right]^2 \right\} \end{aligned} \tag{21}$$

As a result

$$Q^h = \omega \frac{W^{\text{st}}_{\text{int,h}}}{P_{\text{rad,h}}} \tag{22}$$

where index $h$ encodes electric or magnetic multipole.

Expressions (22) are characterized by the Q-factor of the mode in the single multipole approximation. Fig. S3 show good agreement between the analytical expression and the numerical simulation for the electric and magnetic fields, respectively.

Figure 4 in the main paper and Fig. S3 and S4 here shows the Q-factor as a function of $k_b$ at $\Gamma$ point, where we can see that the law of decreasing Q-factor is

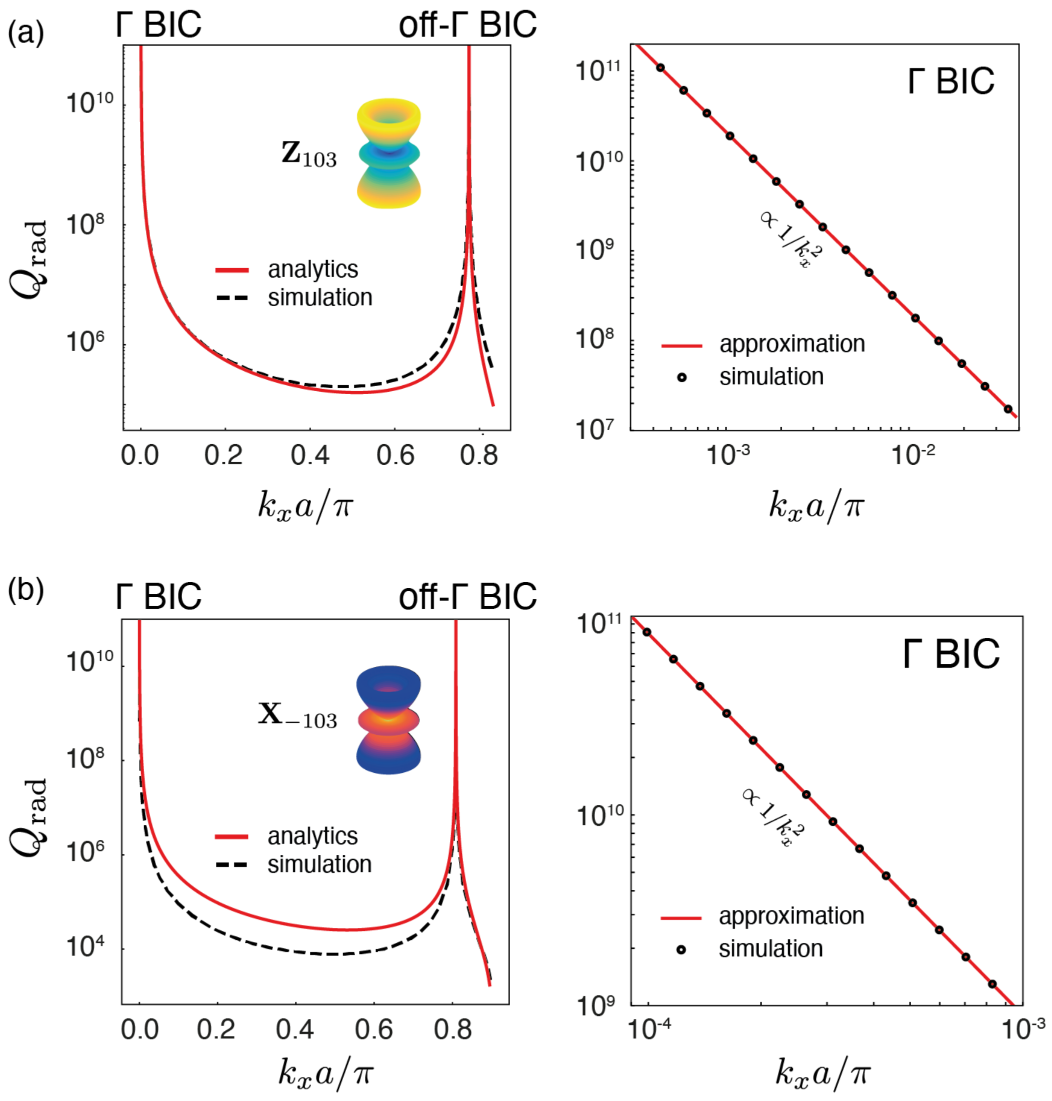


FIG. S3: (a) and (b) Quality factor depenfing on $k_x a/\pi$ for full range of the first zone of Brillouin zone and range in the vicinity of Γ BIC for electric octopole ($\mathbf{Z}_{103}$) and magneteic octopole ($\mathbf{X}_{-103}$), respectively. The permittivities of the sphere are $\varepsilon = 80$ and $\varepsilon = 50$ for electric and magnetic octupolar lattice, respectively.

$$Q \sim \frac{1}{|\mathbf{Y}_s(\frac{\boldsymbol{k}}{k})|^2} \sim \frac{1}{|k_b|^{2|q|}} \tag{23}$$

where $q$ - value of topological charge.

Figure S4 shows that, using the 4th order magnetic multipole as an example, the law of decreasing Q-factor as a function of $k_b$ vector at Γ point is the same in the directions $\Gamma M$ and $\Gamma X$. And it can be proved on the basis of the spherical vector function, due to the separation of variables $\theta$ and $\phi$.

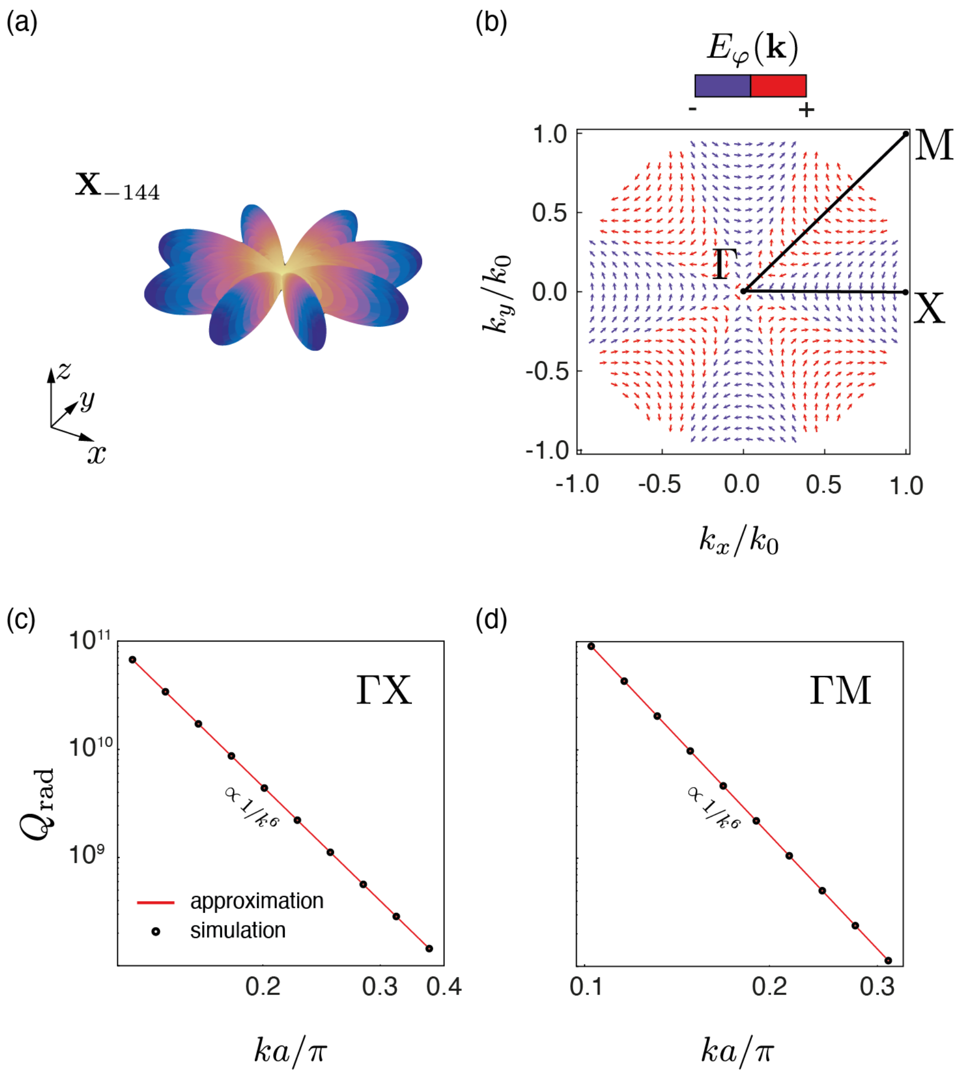


FIG. S4: (a) The far-field radiation of unit cell for magnetic multipole of 4th order. (b) Directions of vector field $\mathbf{E}$ in the k-space (c) and (d) Quality factor $Q$ depenfing on $ka/\pi$ in the directivity $\Gamma X$ and $\Gamma M$, respectivity.

### S4. Far-field and polarization maps of multipolar latices

Using the Bloch theorem for photonic crystals

$$\mathbf{E} = \mathbf{U}\exp(ik_x x + ik_y y) \tag{24}$$

where $\mathbf{U}$ is the field of the unit cell.

$$\mathbf{U} = \mathbf{E}\exp(-ik_x x - ik_y y) \tag{25}$$

$$\mathbf{U} = \sum_{m,n} \mathbf{C}_{m,n}(z)\exp\left(\frac{2\pi imx}{a_x} + \frac{2\pi iny}{a_y}\right) \tag{26}$$

- Fourier series.

$$\mathbf{E}\exp(-ik_x x - ik_y y) = \sum_{m,n} \mathbf{C}_{m,n}(z)\exp\left(\frac{2\pi imx}{a_x} + \frac{2\pi iny}{a_y}\right) \times \int_{a_x}\int_{a_y} ... \exp\left(-\frac{2\pi imx}{a_x} - \frac{2\pi iny}{a_y}\right) dxdy \tag{27}$$

$$\mathbf{C}_{m,n}(z) = \frac{1}{a_x a_y}\int_{a_x}\int_{a_y} \mathbf{E}\exp\left(-i\left(\frac{2\pi m}{a_x} + k_x\right)x - i\left(\frac{2\pi m}{a_y} + k_y\right)y\right) dxdy \tag{28}$$

We work in the subdifraction regime, the only nonzero propagating-wave amplitudes are the zero-order (constant in-plane) Fourier coefficients of $\mathbf{U}$ and $m = n = 0$

$$\mathbf{C}_{0,0}(z) = \frac{1}{a_x a_y}\int_{d_x}\int_{d_y} \mathbf{E}\exp(-ik_x x - ik_y y) dxdy \tag{29}$$

The field outside the multipolar lattice is expressed as follows

$$\boxed{\mathbf{E}(\mathbf{r}) = \frac{S_b}{2\pi k k_z}\exp(i\mathbf{kr})i^{-l}\tilde{D}_s\left[\mathbf{Y}_s\left(\frac{\mathbf{k}}{k}\right)\right]} \tag{30}$$

$$\mathbf{E}(\boldsymbol{k}) = \langle \mathbf{U} \rangle = \mathbf{C}_{0,0}(z) = \frac{S_b}{2\pi k k_z}\exp(ik_z z)i^{-l}\tilde{D}_s\left[\mathbf{Y}_s\left(\frac{\mathbf{k}}{k}\right)\right] \tag{31}$$

The brackets $\langle\cdot\rangle$ denote the spatial average over one unit cell. The electric field $\mathbf{E}(\boldsymbol{k})$ in the k-space is the "polarization vector."

## S5. Anapole state in the multipolar lattice

Figure S5(a) demonstrates the reflection map $R$ from the multipolar lattice composed of electric octupoles $\mathbf{Z}_{103}$. The at-$\Gamma$ and off-$\Gamma$ BICs are formed at the points of intersection of the modes and the lines $\theta = 0$ and $\theta = \theta_0$, respectively. However, there is an anapole state in this multipolar lattice, where the lattice does not interact with the incident field and the lattice becomes completely transparent. The collective anapole states has no dispersion and its frequency ($\omega a/2\pi c = 0.4365$) coincides with the anapole in a single particle as the multipoles do not interact via scattering in the anapole regime. Figure S5(b) shows the normalized scattering cross section $C_{sca}/S$ as a function of $\omega a/2\pi c$ which demonstrates that the frequency of the lattice anapole coincides with the frequency of anapole in the single dielectric sphere.

## S6. NUMERICAL SIMULATIONS

MULTEM ([3, 4]) is an open-source software for calculating light transmission, reflection, and absorption coefficients of 2D periodic infinite lattices. We used MULTEM to calculate the reflection map $R$ as a function of frequency $\omega$ and angle of incidence $\theta$, see Figs. 1(c), 2, and 3(b) in the main paper and Figs. S2(b), S2(b) and S5. We modified the original code using 1) an MIT implementation of Faddeeeva function [5] and 2) the LAPACK library to solve the system of linear equations. We also introduced a simulation of a multipolar lattice (see details below). A modified version of MULTEM is available at [6].

We use multipoles of a specific type, angular momentum, and projection of angular momentum to construct a 2D multipole lattice, which was achieved by nullifying all other multipole T-matrix coefficients in the original MULTEM subroutines SETUP and PCSLAB. The internal field of each cell $\mathbf{E}^{in}$ consists of only one vector spherical harmonic, which is oriented along the $z$ axis. Subroutine PCSLAB computes the transmission and reflection matrices for a plane of spheres embedded in a homogeneous host medium. PCSLAB solves the system of linear equations (32) which gives the scattered field coefficients $b_{lm}^{+P}$ in terms of the incident field coefficients $a_{lm}^{0P}$.

$$\begin{pmatrix} \mathbf{I} - \mathbf{T}^E\mathbf{\Omega}^{EE} & \mathbf{T}^E\mathbf{\Omega}^{EH} \\ \mathbf{T}^H\mathbf{\Omega}^{HE} & \mathbf{I} - \mathbf{T}^H\mathbf{\Omega}^{HH} \end{pmatrix} \begin{pmatrix} \mathbf{b}^{+E} \\ \mathbf{b}^{+H} \end{pmatrix} = \begin{pmatrix} \mathbf{T}^E\mathbf{a}^{0E} \\ \mathbf{T}^H\mathbf{a}^{0H} \end{pmatrix}, \tag{32}$$

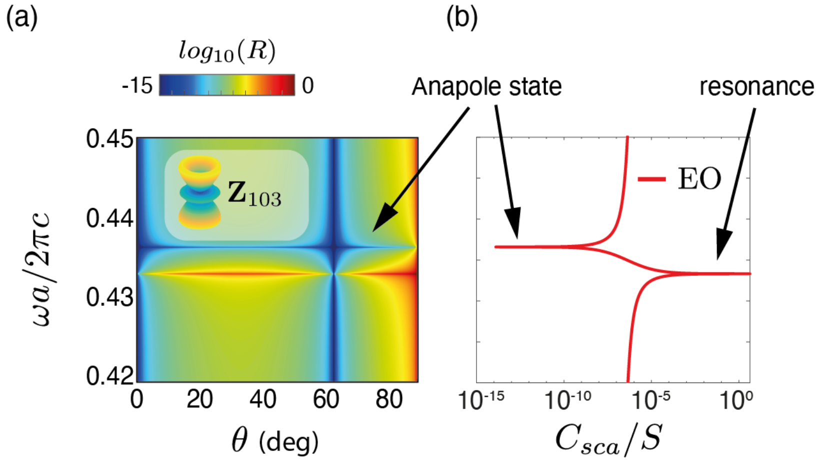


FIG. S5: (a) The reflection R from the electric octupolar lattice with a square plotted as a function of dimensionless frequency $\omega a/2$ and angle of incidence $\theta$ for the ration $a/d = 1.75$ in logarithmic scale. (b) Normalized scattering cross-section $C_{sca}/S$ depending on $\omega a/2\pi c$ for single dielectric nanosphere

where $\mathbf{I}$ is the $l_{max}(l_{max}+2) \times l_{max}(l_{max}+2)$ unit matrix, $\mathbf{T}^P$ is the diagonal of sphere T-matrix, and $\mathbf{\Omega}^{PP'}$ are the coupling matrices of the scattered field coefficients from a single sphere $b_{lm}^{+P}$ and the scattered field coefficients from all others spheres in lattice $b_{lm}^{\prime P}$, where $P$ is the multipole type (electric or magnetic).

Subroutine SETUP constructs the square matrices on the left-hand sides of expression (32) and stores them in the arrays XXMAT1 and XXMAT2. For this purpose it uses the diagonal of a single sphere T-matrix computed by subroutine TMTRX and stored in arrays TE and TH. To consider the contribution of one electric or magnetic multipole to the reflection, we leave one non-zero element in the TE or TH arrays correspondingly. The right-hand side is stored in arrays BMEL1 and BMEL2 which are formed in subroutine PCSLAB using the modified arrays TE and TH. See [3] for more details.

We extracted the Q-factor from the calculated reflectance spectra using the generalized Fano resonance formula [7]. Figure 4 in the main paper and Fig. S3 and S4 here show the Q-factor as a function of $k$ vector projection $k_x$.

Maps of electric field $\mathbf{E}(\boldsymbol{k})$ in the k-space for Fig. 3c, 4 in the main paper and Fig. S2(c,e) and S4b here were calculated in Wolfram Mathematica and plotted in Python.

Normalized scattering cross section of single isotropic sphere was calculated using Mie calculator [8].

---

* Electronic address: a.bogdanov@metalab.itmo.ru

[1] J. A. Stratton, *Electromagnetic theory*, vol. 33 (John Wiley & Sons, 2007).
[2] C. F. Bohren and D. R. Huffman, *Absorption and scattering of light by small particles* (John Wiley & Sons, 2008).
[3] N. Stefanou, V. Yannopapas, and A. Modinos, Computer physics communications **113**, 49 (1998).
[4] V. Y. N. Stefanou and A. Modinos, *Multem* (1998), URL http://cpc.cs.qub.ac.uk/summaries/ADIM_v2_0.html.
[5] S. G. Johnson, *Faddeeva package*, URL http://ab-initio.mit.edu/wiki/index.php/Faddeeva_Package.
[6] K. Ladutenko and A. Shalev, *Multem (modified version)* (2021), URL https://github.com/wave-scattering/amos-try.
[7] A. A. Bogdanov, K. L. Koshelev, P. V. Kapitanova, M. V. Rybin, S. A. Gladyshev, Z. F. Sadrieva, K. B. Samusev, Y. S. Kivshar, and M. F. Limonov, Advanced Photonics **1**, 016001 (2019).
[8] K. Ladutenko, *Mie calculator*, URL https://physics.itmo.ru/en/mie#/spectrum.
